# Supplementary material for: Vibrational signatures for the identification of single-photon emitters in hexagonal boron nitride
Source: arXiv:2008.05817 source file (2021-01-13)
Supplement: Supplementary file 1 [file supplementary-information.pdf]

# Supplementary Information: Vibrational signatures for the identification of single-photon emitters in hexagonal boron nitride

Christopher Linderälv,[1] Witlef Wieczorek,[2] and Paul Erhart[1]

[1] *Chalmers University of Technology, Department of Physics, Gothenburg, Sweden*

[2] *Chalmers University of Technology, Department of Microtechnology and Nanoscience, Gothenburg, Sweden*

## I. VIBRATIONAL PROPERTIES OF DEFECT STRUCTURES

In Fig. S1, the energy landscape for displacing the C atom perpendicular to the h-BN plane is shown. $C_B$-$V_N$ in a singlet electron configuration is dynamically unstable. The $C_B$ (neutral) defect exhibits a very flat energy landscape upon displacement perpendicular to the h-BN plane, which results in small imaginary frequencies in the phonon spectrum that are not associated with a lower energy structure.

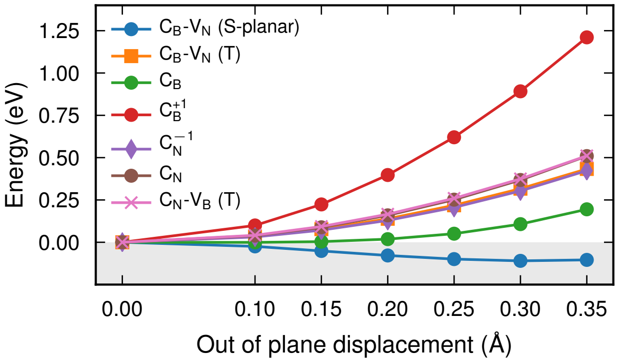


FIG. S1. Energy landscape as a function of out-of-plane displacement of the C atom for C impurity defects.

## II. IDEAL VS. DEFECT PHONON MODES

The spectral distribution function for the charged transition on $C_N$ and the charge neutral transition on $C_B$-$V_N$(T) is shown in Fig. S2. The $C_N$ defect geometry is similar to the pristine h-BN and there are no obvious local modes (low inverse participation ratio) with large influence on the lineshape. For $C_B$-$V_N$(T), approximating the lineshape with bulk phonon modes results in a quite poor approximation likely because the vacancy induces relatively large structural differences. The vacancy atom is accounted for by adding an atom to the $C_B$-$V_N$(T) structures at the same place so that the contribution from the vacancy to the Huang-Rhys (HR) factor is zero.

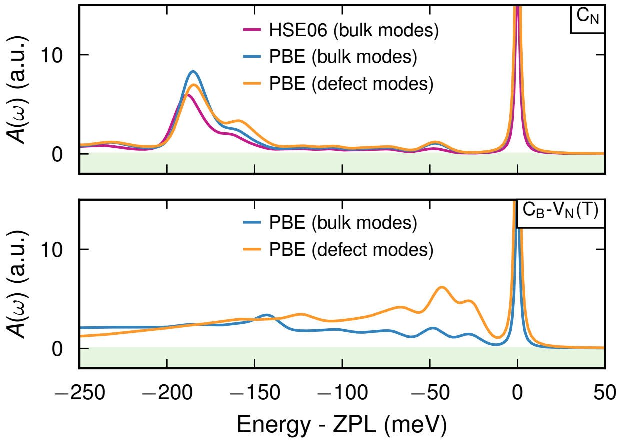


FIG. S2. Lineshape function $A(\omega)$ for $C_N$ (top) and $C_B$-$V_N$ (T; bottom) computed using either defect or bulk phonon spectra.

## III. DISSOCIATED $C_N$-$C_B$

In Fig. S3a, the formation energy diagram as computed with PBE is shown. Also, the HSE06 band edges are superimposed to obtain an estimate of the charge transition level (CTL) with a better band gap description. The spectral distribution function of the (+1/0) transition for various distances is shown in Fig. S3b.

## IV. SINGLET VS. TRIPLET STATE IN $C_B$-$V_N$

The analysis of the singlet and triplet state stability has been performed on a $7 \times 7 \times 1$ cell with a 500 eV plane wave cutoff energy. In Fig. S4 the 1D configuration coordinate diagram between the singlet and triplet states of the $C_B$-$V_N$ defect is shown. At the triplet geometry the triplet state is stable, but the energy between the crossing point of the singlet and triplet state is very close to the triplet energy at the equilibrium geometry.

In Fig. S5 the energy difference between the triplet and singlet state of charge neutral $C_B$-$V_N$ is shown. The LDA functional predicts a stable triplet state while PBE, PBEsol, rPBE and HSE06 places the triplet state lower in energy.

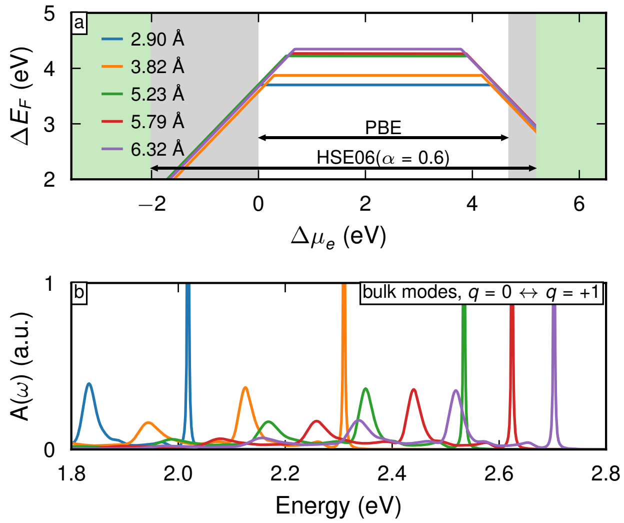


FIG. S3. a) Formation energies of dissociated $C_B$-$C_N$ defects. b) Spectral distribution function for the +1/0 charge transition.

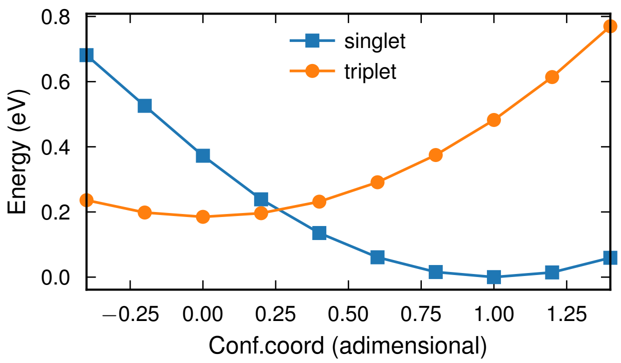


FIG. S4. Energy landscape for ($C_B$-$V_N$) obtained by interpolation between the equilibrium configurations for the planar singlet and triplet states.

## V. CONVERGENCE OF SPECTRAL DISTRIBUTION FUNCTION

The convergence of the spectral distribution function $A(\omega)$ for a set of different computational parameters relating to the integration in time is shown in Fig. S6.

## VI. KOHN-SHAM STATES FOR DEFECTS

In Fig. S7 the Kohn-Sham states for the neutral charge states of the considered defects are shown. The band edges from the primitive structure are superimposed.

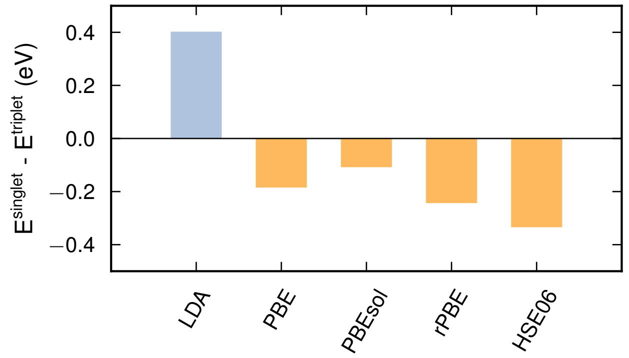


FIG. S5. Energy difference between the planar singlet and triplet states of ($C_B$-$V_N$) for various functionals. For HSE06, the computation was performed with the standard mixing parameter.

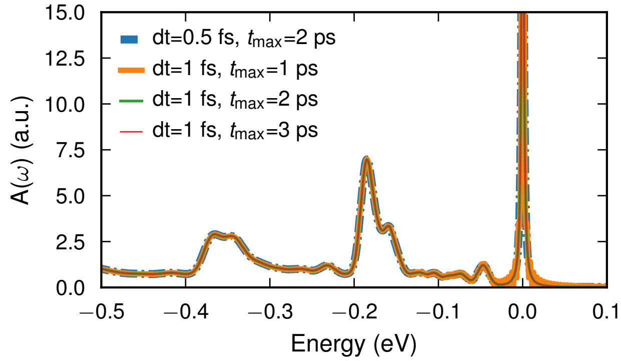


FIG. S6. The convergence of the spectral distribution function for the case of $C_N$.

## VII. SPECTRAL FUNCTION AND DISTRIBUTION

In Fig. S8, the spectral distribution function is shown for the defects $C_N$, $C_B$, $C_B$-$V_N$(T), $C_B$-$C_N$ evaluated with phonons from the defect structure. In Fig. S9, the spectral function for the defects in Fig. S8 is shown.

In Fig. S10, the supercell size effect of the electron-phonon spectral function and the resulting spectral distribution function is shown for the charged transition on $C_N$. The agreement is very good albeit some minor differences can be seen, specially for low frequencies.

The influence of the damping parameter $\kappa$ is shown in Fig. S11.

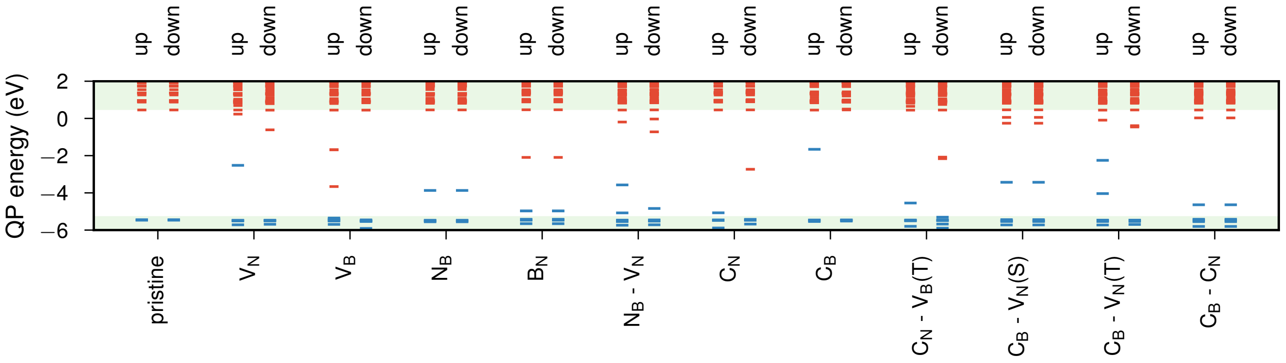


FIG. S7. Kohn-Sham states for the neutral charge state of the considered defects computed with HSE06 ($\alpha = 0.25$).

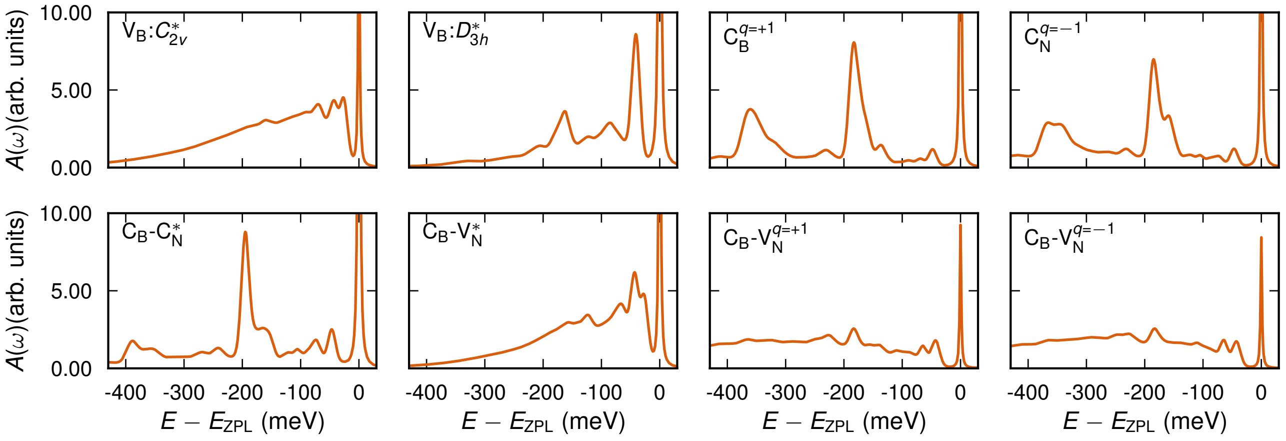


FIG. S8. Lineshape function $A(\omega)$ for a set of defects.

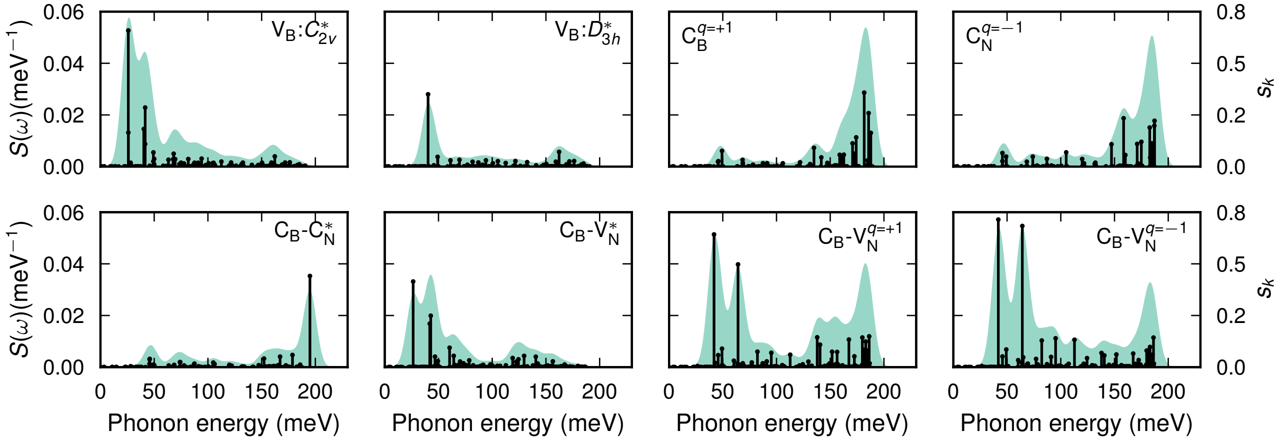


FIG. S9. Spectral function $S(\omega)$ for a set of defects.

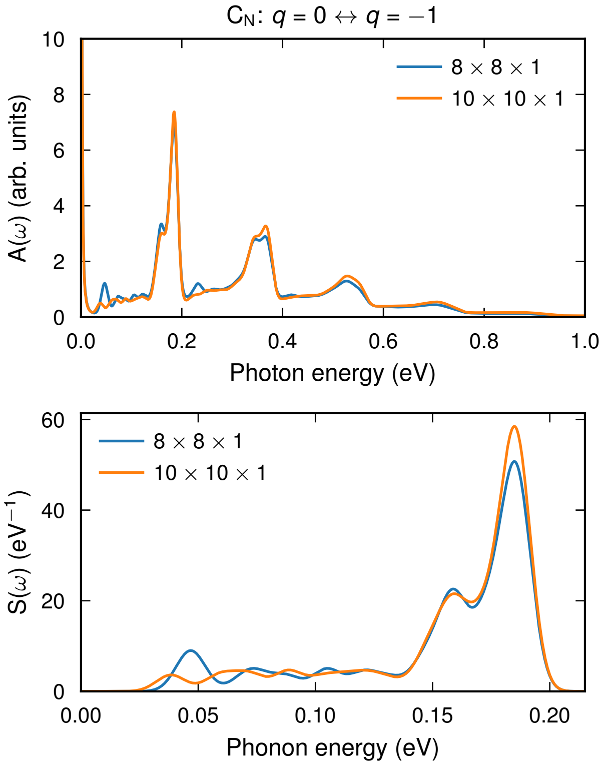


FIG. S10. Spectral distribution function $A(\omega)$ and electron-phonon spectral function $S(\omega)$ for the charged transition on $C_N$ as computed using two different supercell sizes.

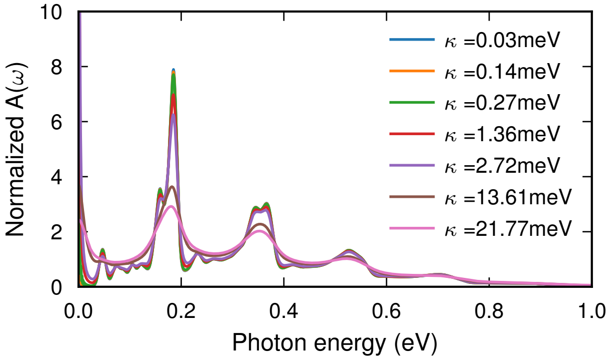


FIG. S11. Effect of the broadening parameter $\kappa$ on the spectral distribution function $A(\omega)$ for the charged transition on $C_N$.
